# Supplementary material for: Extreme thermodynamics with polymer gel tori: harnessing thermodynamic instabilities to induce large-scale deformations
Source: arXiv:1806.11049 ancillary file (2018-06-28)
Supplement: Supplementary file 1 [file SI-arxiv.pdf]

# Supplementary Information

June 28, 2018

## 1 Generation of toroidal hydrogels and details of the quasistatic deswelling experiments

We fabricate toroidal gels by first forming toroidal droplets of a precursor solution consisting 5% NIPAM, 0.2% crosslinker bis-acrylamide, 0.2% (w/v) photo-initiator Irgacure 2959, and 94.6% deionized water, inside a yield-stress material made of a mixture of Dow Corning® 9041 silicone elastomer blend and 10cst silicone oil [1]. The process consists of injecting the precursor fluid through a needle into a rotating bath containing the yield-stress material. At sufficiently high rotation speeds, the stresses involved exceed the yield stress, and we can successfully generate a curved jet that closes onto itself to form a toroidal droplet. Once made, the shape is stabilized by the elasticity of the yield-stress material [2]. We induce polymerization of the precursor fluid by illuminating the sample with UV-light while keeping it over an ice bath, which assists with heat dissipation and prevents macro-phase separation of pNIPAM aggregates during polymerization. The resultant toroidal gel is removed from the yield-stress material by repeated cleaning with alcohol and water, and maintained in deionized water.

Quasistatic deswelling experiments are performed by transferring a fully swollen gel into a water bath that is placed over a platform with temperature control capability; the temperature of the bath is measured using a thermocouple of sensitivity $\pm 0.1$ °C. The volume and shape transition of the toroidal gel are monitored using a CCD camera. To ensure quasistatic deswelling, we change the temperature at a rate $\leq 0.4$ °C/hour. Alternatively, we change the temperature in small steps, waiting as needed after each step until no size change is detected; the results we observe are identical. We also emphasize that the deswelling behavior is fully reversible.

## 2 Simulation information

In our computational model, we utilized dissipative particle dynamics (DPD), a particle-based mesoscopic simulation technique, whose soft potentials and pairwise forces preserve local hydrodynamics while allowing for simulations with longer length and time scales [3, 4, 5]. The governing dynamics between beads in DPD are set by three main forces, $\mathbf{F} = \sum_{j\neq i} \mathbf{F_{ij}^C} + \mathbf{F_{ij}^D} + \mathbf{F_{ij}^R}$. The conservative force $\mathbf{F_{ij}^C} = a_{ij}\, w(r_{ij})\, \mathbf{\hat{r}_{ij}}$ leads to excluded volume. In this expression, $a_{ij}$ is the repulsion parameter between beads $i$ and $j$, and $w(r_{ij}) = 1 - \hat{r}_{ij}$ is a weighing function, where $\hat{r}_{ij} = r_{ij}/r_C$, with $r_{ij} = |\mathbf{r_i} - \mathbf{r_j}|$ and $r_C$ the cut-off distance of the excluded volume potential. The dissipative force $\mathbf{F_{ij}^D} = -\gamma\, w^2(r_{ij})\, (\mathbf{\hat{r}_{ij}} \cdot \mathbf{v_{ij}})\, \mathbf{\hat{r}_{ij}}$, with $\mathbf{v_{ij}}$ the difference in velocity between beads $i$ and $j$, accounts for viscous interactions, while the random force $\mathbf{F_{ij}^R} = \sigma\, w(r_{ij})\, \xi_{ij} \cdot (\Delta t)^{-1/2}\, \mathbf{\hat{r}_{ij}}$ represents the effect of thermal fluctuations. In the expression for $\mathbf{F_{ij}^R}$, $\xi_{ij}$ is a standard normal variable with zero mean and $\Delta t$ is the time-step of the velocity verlet algorithm; the time-step dependence is required to guarantee that Brownian motion, which is characterized by a magnitude of the displacement-step that scales with the square-root of the time-step, is recovered upon integration. The random and dissipative forces are related by $\sigma^2 = 2\,\gamma\, k_B\, T$, with $k_B$ the Boltzmann constant and $T$ the temperature, due to the fluctuation-dissipation theorem. For our simulations, we set $a_{ij} = 25$, $r_C = 1$, $\gamma = 4.5$, $k_B\, T = 1$, and $\rho = 3$ (all dimensional parameters are given in DPD units) [3].

We developed two different toroidal gel models to describe the slow and rapid heating rates in the experiments. For slow heating rates, we represent the toroidal polymer network using randomly connected

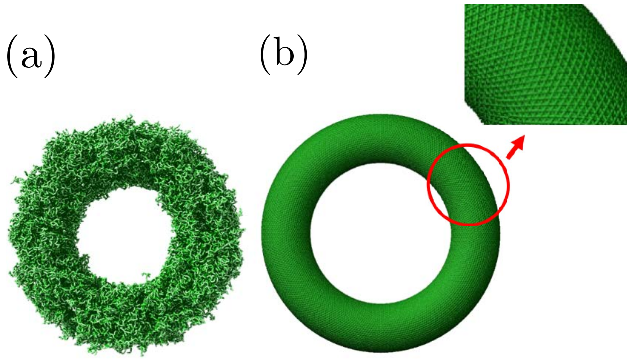


Figure S.1: (a) Example image of a toroidal polymer network used to model quasistatic deswelling. (b) Illustration of a toroidal mesh with close-up, used to model the rapid heating rate experiments.

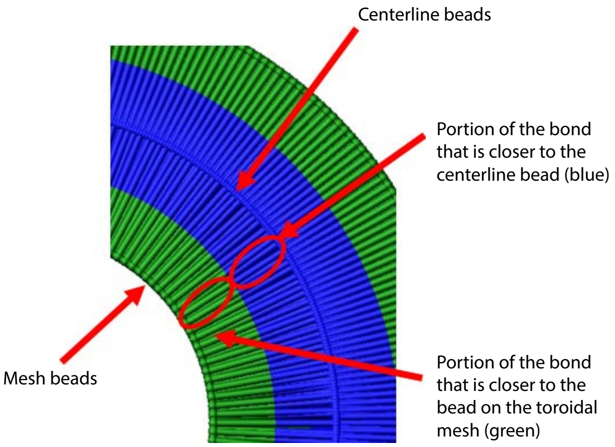


Figure S.2: Cross-sectional view of toroids for rapid heating simulations. The beads in the toroidal mesh and centerline beads are shown in green and blue, respectively. Each mesh-centerline bond is represented with a half-green and a half-blue color scheme for illustration purposes.

bead-spring chains. In this approach, the flexible chains are composed of beads connected by a harmonic potential given by $U_{\text{bond}} = k_{\text{bond}}\,(r - r_{\text{eq}})^2$ and a bending potential given by $U_{\text{bend}} = k_{\text{bend}}\,(1 + \cos\theta)$. Here, $k_{\text{bond}}$ is the bond stiffness, $r_{\text{eq}}$ is the equilibrium separation length between beads, $k_{\text{bend}}$ is the bending stiffness and $\theta$ is the angle between two polymer bonds sharing a common bead. In our simulations, we set $k_{\text{bond}} = 35$, $r_{\text{eq}} = 0.6$, and $k_{\text{bend}} = 1$. To construct our toroidal gel network, we randomly distribute crosslink points in a $60 \times 60 \times 60$ simulation domain and then connect them with nearby neighbors via flexible chains using a connectivity of 6. The toroidal geometries are cut out from the corresponding cubic networks and placed in a $100 \times 100 \times 100$ simulation domain filled with a viscous solvent with density $\rho = 3$ represented by DPD beads. Deswelling of toroidal gels is achieved by varying the gel-solvent repulsion parameter $a_{N-S}$ [6]. Theta-solvent conditions correspond to $a_{N-S} = 25$. Lower values of $a_{N-S}$ correspond to good solvent and higher values correspond to poor solvent conditions. To model the collapse of the toroidal gel, we start at theta-solvent conditions and incrementally decrease the solvency until we reach $a_{N-S} = 35$. Figure S.1a shows a snapshot of our toroidal network in theta-solvent conditions. The swelling kinetics of our random polymer network model, in the case of spherical geometries, agrees well with Tanaka's theory for the swelling of gels [6, 7].

Due to computational constraints, our gel model cannot be directly used to model the rapid heating rate experiments with macroscopic gels, which is characterized by the formation of a dense, stiff skin at the gel-solvent interface. To model the effects of the stiff gel skin which forms in these cases, we use a simplified

model that is composed of a toroidal shell constructed using a tetrahedral mesh with an average spacing of ∼0.35, as shown in Fig. S.1b. Nodes in the mesh are connected by harmonic bonds. To mimic the effect of the gel heating rate, we arrange beads along the toroidal centerline and connect them to the beads forming the shell. Mesh-centerline bonds are shown in the cross-sectional view in Fig. S.2, where half of each bond is colored in blue (parts closer to the centerline bead) and the other half is colored in green (portion of the bond closer to the mesh bead). The initial equilibrium bond length for the mesh-centerline bonds was set to 5. The harmonic bonds in the shell have stiffness $k = 500$, while the mesh-centerline harmonic bonds have stiffness $k = 100$. Note that we do not impose a DPD repulsion between the beads in the mesh, as this would have effects on the mesh properties that we want to avoid. The repulsion between mesh-solvent beads is $a_{M-S} = 100$. The density of the fluid is $\rho = 3$, yielding an average spacing between solvent beads of about 0.7. The smaller spacing between beads in the mesh and the relatively large repulsion between mesh-solvent beads ensures that solvent particles which are initially inside of the toroidal mesh remain trapped during the rapid heating process. To model this rapid heating, we instantaneously decrease the mesh-centerline equilibrium bond length from 5 to 3. The final bond length is selected based on the numerical stability of the shell model.

# 3 Comparison between simulation and Pringle$^{\text{TM}}$ shape

We compare the simulation results to the Pringle$^{\text{TM}}$ shape predicted by our elastic ring model by fitting the simulated centerline, an example of which is shown in Fig. S.3(a) below, to a ring that lies on a hyperbolic paraboloid $z = q\,(x^2 - y^2)$, which, in polar coordinates is given by

$$(x,\, y,\, z) = R\left(\cos(\theta+\delta),\, \sin(\theta+\delta),\, q\,R\,\cos(2\theta+\delta)\right), \tag{1}$$

where $R$ is the radius of the projection of the ring onto the $xy$-plane, $\delta$ is a phase-offset, and $q$ determines the amplitude of the out-of-plane component of the buckled ring. To perform this fit, we first translate and rotate the simulated points such that (i) the origin $x, y, z = 0$ coincides with their center-of-mass and (ii) the $z$-axis aligns with the principle axis corresponding to their smallest dimension. Next, we fit the projected ring radius $R$ against the projection of the simulated centerline to the $xy$-plane. Using this value of $R$, we fit $q\,R^2\,\cos(2\theta+\delta)$ to the $z$-axis projection of the centerline, as shown in Fig. S.3(b), obtaining values of $A = q\,R^2$ and the phase-offset $\delta$. For the specific case shown in this figure, we obtain an amplitude of $A/R \approx 0.068$ and $\delta \approx 0.242$ radians. As evidenced by Figs. S.3(b,c), the buckled shape is well-approximated by a ring on a hyperbolic paraboloid, i.e., the Pringle$^{\text{TM}}$ shape.

We note that since we lack a three-dimensional view of the toroids in the experiments, we cannot provide a similar quantitative analysis of the observed, buckled Pringle-like shape.

# 4 Phase coexistence in a gel rod

To address the phase-coexistence between solvent-poor (deswollen) shell and solvent-rich (swollen) interior, we approximate the toroid by a cylinder with identified end-caps; the toroid's ring curvature lifts the cylinder's polar symmetry. In the absence of ring curvature, symmetry dictates that the cylinder can only change its length by a stretching factor $\Lambda_\ell$, the radius of the solvent-rich region by a factor $\Lambda_t$, and the thickness of the solvent-poor region by $\Lambda_n$. This situation is illustrated in Fig. S.4. The total free-energy, in the reference space $\mathcal{R}$, is given by

$$\begin{aligned}\frac{F}{\pi\,a^2} =&(1-f)\left[\frac{1}{2}\,\mu_0\,\left(\Lambda_\ell^2 + 2\,\frac{\phi_0}{\phi_r\,\Lambda_\ell}\right) + \mathcal{F}(\phi_r)\right]\\ &+ f\,\left[\frac{1}{2}\,\mu_0\,\left(\Lambda_\ell^2 + \phi_0\,\frac{\phi_p^{-2}+\phi_r^{-2}}{\phi_r^{-1}\,\Lambda_\ell}\right) + \mathcal{F}(\phi_p)\right]\\ &+ p\,\left[(1-f)\frac{\phi_0}{\phi_r} + f\,\frac{\phi_0}{\phi_p} - 1\right]\end{aligned} \tag{2}$$

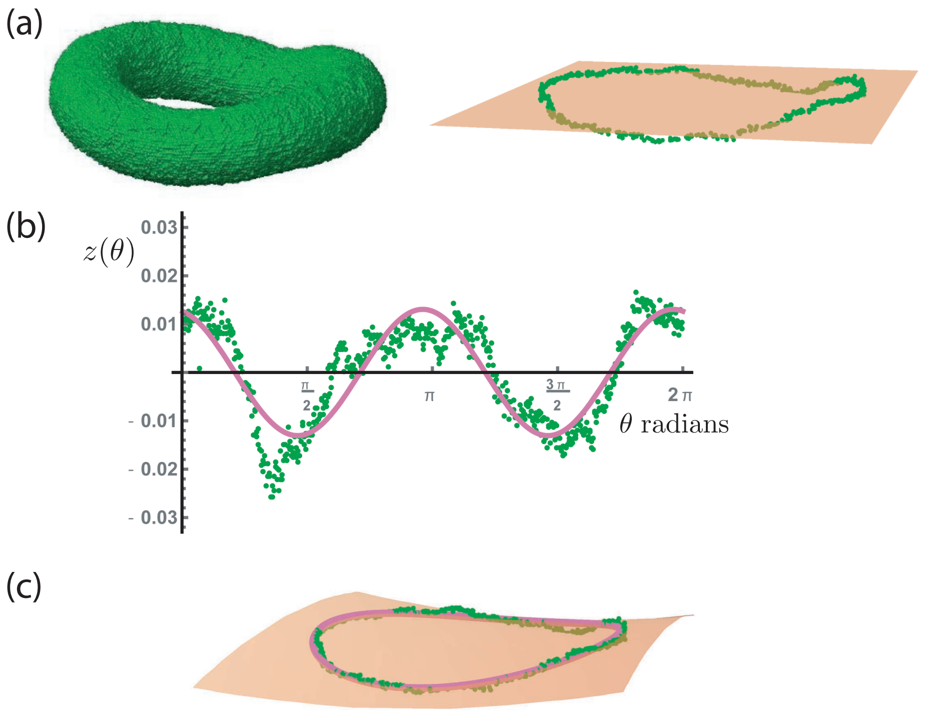


Figure S.3: (a) Buckled shape from DPD simulation, with extracted centerline (right) and $xy$-plane. (b) Height of the ring as measured along the $z$-axis of (a), together with a fit to $A\cos(2\theta+\delta)$, where $A = q\,R^2$ is the amplitude of the ring deformation and $\delta$ is a phase offset, accounting for the choice orientation in the $xy$-plane; in this example, we find $\delta \approx 0.242$ (radians) and $A/R \approx 0.068$. (c) Overlay of the data with the fit ring on a portion of the corresponding hyperbolic paraboloid surface.

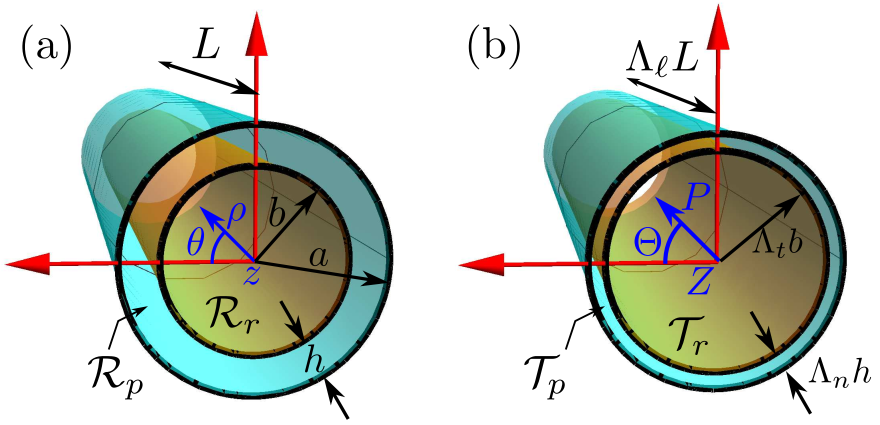


Figure S.4: Schematic of phase-separated cylinder (a) before and (b) after deformation along with cylindrical coordinates. In the reference configuration (a), $L$ is the length of the cylinder, $b$ is the radius of the solvent-rich region, $h$ is the thickness of the solvent-poor skin, $\mathcal{R}_r$ is the solvent-rich region, $\mathcal{R}_p$ is the solvent-poor region. $\mathcal{T}_r$ is the solvent-rich region and $\mathcal{T}_p$ is the solvent-poor region in the target configuration (b).

where $\mu_0$ is the shear rigidity of the gel before phase-separation, with polymer volume fraction $\phi_0$; after phase-separation, the gel has a solvent-poor shell with polymer volume fraction $\phi_p^{-1} = \Lambda_n \Lambda_t \Lambda_\ell \phi_0^{-1}$ and solvent-rich interior with polymer volume fraction $\phi_r^{-1} = \Lambda_t^2 \Lambda_\ell \phi_0^{-1}$. The parameter $p$ is a Lagrange multiplier that enforces the constant volume condition. The mixing free energy density $\mathcal{F}$ is modeled by the Flory-Rehner theory [8, 9]; for description of the continuum approach, see e.g. [10]. In order to describe the first-order phase transition that occurs in the neutral polyNIPAM gels, the Flory-Rehner theory is extended via a virial expansion of the osmotic pressure [11], leading to a volume fraction-dependent Flory parameter, which may be approximated as

$$\chi(\phi, T) \approx \chi_1(T) + \chi_2\, \phi \tag{3}$$

where $\chi_2$ is typically taken to be fixed by experiment with a value $\chi_2 > 1/3$ [12]; temperature sets the value of $\chi_1$ which determines the swelling state of the gel. Minimizing the total free-energy Eq.2 with respect to $\phi_r$, $\phi_p$, $\Lambda_\ell$ gives stress-balance conditions; minimization with respect to $f$ yields a chemical potential-balance condition between the two phases; minimization with respect to $p$ yields the "lever rule"

$$f = \frac{\phi_r^{-1} - \phi_0^{-1}}{\phi_r^{-1} - \phi_p^{-1}} \tag{4}$$

which is simply a consequence of mass and volume conservation and thus holds for systems undergoing phase separation into two distinct phases [13]. Note that in the manuscript, in order to clarify the form of our elastic model, we introduce the strains $u_r$ and $u_p$ where

$$u_r \equiv \frac{\phi_0 - \phi_r}{\phi_r}; \quad u_p \equiv \frac{\phi_0 - \phi_p}{\phi_p} \tag{5}$$

which allows the lever rule Eq. 4 to be recast as

$$f = \frac{u_r}{u_r - u_p}\,. \tag{6}$$

Fig. S.5 outlines the theoretical predictions for the equilibrium state of a long cylindrical gel, with fixed solvent and polymer mass, as a function of Flory parameter $\chi_1$, which is a proxy for temperature. In particular, we focus on gels that contain a much greater mass of solvent than polymer, characterized by a low single-phase polymer volume fraction $\phi_0$, and consider three cases of polymer dilution: $\phi_0 = 0.01$, 0.015, and 0.02. We use representative values $\mu_0 = 10^{-4} k_B T/v$ and $\chi_2 = 0.56$ (see [12]). Equilibrium values of the polymer volume fraction are shown in Fig. S.5(a), where we note that for small $\chi_1$, there is a single

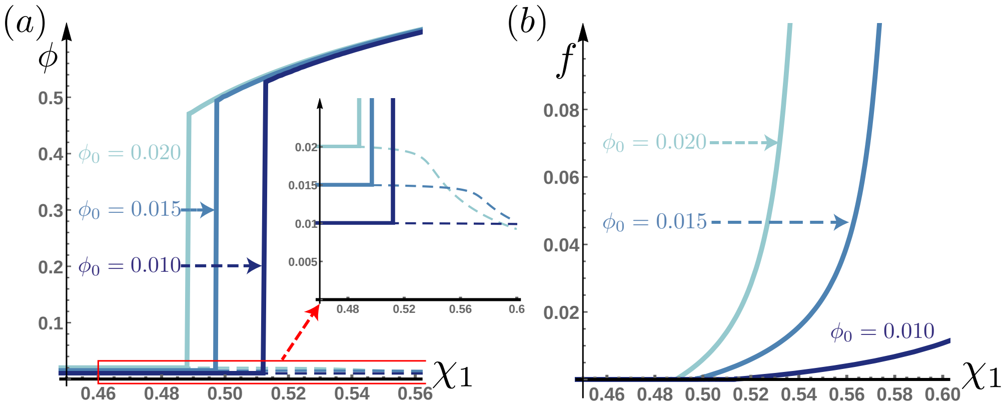


Figure S.5: (a) Values of solvent-poor volume fraction $\phi_p$ (solid) and solvent-rich volume fraction $\phi_r$ (dashed) after constrained phase separation are shown as a function of $\chi_1$, with inset highlighting the low-$\phi$ regime, showing variation in the solvent-rich volume fraction $\phi_r$. (b) Fraction $f$ of solvent-poor phase in the reference state is shown as a function of $\chi_1$.

equilibrium volume fraction, given by $\phi_0$, and for larger $\chi_1$, the gel phase-separates and the equilibrium state is characterized by coexistent solvent-rich and solvent-poor phases with volume fractions $\phi_r$ (dashed curve) and $\phi_p$ (solid curve), respectively. Thus, the gel undergoes a first-order deswelling phase transition resulting in the large, discontinuous jump in $\phi_p$ from $\phi_0$. We find, however, that the solvent-rich region is characterized by a volume fraction $\phi_r$ that decreases continuously from $\phi_0$; this is emphasized in the inset of Fig. S.5(a), which focuses on a smaller range of volume-fraction and a larger range of $\chi_1$ to highlight the variation in $\phi_r$. Note that for more dilute gels (lower $\phi_0$), the phase-separation transition occurs at higher $\chi_1$ and variation of $\phi_r$ from $\phi_0$ is diminished. We emphasize, though, that there is still a variation in $\phi_r$ from $\phi_0$ for the case of $\phi_0 = 0.01$; this variation is apparent after zooming in appropriately.

To better understand the behavior of the phase-separated volume fractions, refer to Fig. S.5(b), which shows the fraction $f$ of the cylinder that is occupied by solvent-poor gel. Since the solvent-poor region grows from the deswollen boundary of the cylinder, rather than the core, where it would need to grow from a critical nucleus, $f$ grows continuously from 0. Within this picture, the solvent-poor region obtains more polymer mass from the solvent-rich region in order to grow, decreasing the polymer volume fraction $\phi_r$ of the solvent-rich region; this decrease is continuous because the growth of $f$ is continuous. The observed increase in the rate of change of $\phi_r$ in the inset of Fig. S.5(a) and of $f$ in Fig. S.5(b) with larger values of $\chi_1$ can be explained by recalling that phase-separation in gels is different from phase-separation in fluids due to the presence of shear rigidity: the formation of separate phases results in an inhomogeneous strain of the polymer network, resulting in a free-energy cost, which limits the growth of separate phases. However, since the elastic modulus $\mu_0$ is independent of $\chi_1$, for sufficiently large $\chi_1$ (sufficiently poor solvent), the portion of the free-energy density due to solvent-polymer mixing overwhelms the elastic part of the free-energy density. As a result, the limiting role of polymer network rigidity in the growth of the solvent-poor phase becomes progressively less important, leading to the increased rate of change of $f$ with $\chi_1$, and the associated increased change in $\phi_r$.

Finally, the shift of the transition value of $\chi_1$ to lower values with increasing $\phi_0$ is due to the correspondingly higher energy density of solvent-polymer mixing with increasing $\phi_0$: for increasing values of $\phi_0$ (in the regime of $\phi_0 \ll 0.5$), there is increasing contact between polymer and solvent molecules (with maximum mixing at $\phi_0 = 0.5$). Thus, the effect of solvent-quality change is greater, resulting in a lower transition value of $\chi_1$, as well as a greater rate of change in $\phi_r$ and $f$ with increasing $\chi_1$.

We also emphasize that our model holds in the low $f$ limit, which is our case, since for larger values of $f$, we would not be able to treat the skin as an elastic shell and would have to resort to solving the continuum equilibrium equations. (We note that $f \approx 0.1$ is consistent with the magnitude predicted by our cylinder model.)

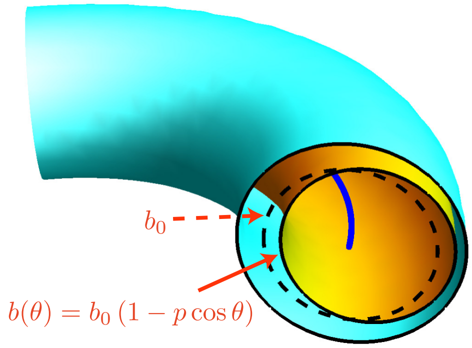


Figure S.6: Adding curvature to the gel cylinder necessitates a *polarization* $p$ of the solvent distribution, described as a displacement of the interface between coexistent regions as shown above.

# 5 Phase separation in tori: introducing ring curvature as a perturbative correction

To determine the effect of the toroid's ring curvature on the phase coexistence, we start with the above cylindrical core-shell model and add the effect of ring curvature $\kappa = 1/R$ *perturbatively.* Note that adding the ring curvature lifts the axial symmetry of the cylinder. As a result, we may no longer assume that the solvent-poor skin has as uniform thickness as a function of the angular coordinate $\theta$; in general, the thickness varies as a function of $\theta$. Equivalently, the position of the interface between solvent-rich and solvent-poor regions is no longer at a fixed radius, viz. $\rho = b$ in the polar coordinates of Fig. S.5. In general, the interface position may be decomposed in Fourier modes as $b(\theta) = b_0 + b_1 \exp i\theta + b_2 \exp 2i\theta + \ldots$, where $b_n$ denotes the amplitude of the $n^{\text{th}}$ mode. However, in analogy with the multipole expansion of the scalar potential in electrostatics, the expansion of $b(\theta)$ can be expressed in terms of multipole moments; for example, $b_0$ characterizes a scalar "charge," $b_1$ a vector "polarization," $b_2$ a rank-2 tensor "quadrupole," etc. Note that the curvature is a vector quantity $\boldsymbol{\kappa} = \kappa\hat{\mathbf{b}}$, where $\hat{\mathbf{b}}$ is the centerline's binormal direction. Therefore, the lowest-order term in the free-energy of the gel ring that incorporates coupling between curvature and interface shape $b(\theta)$ is a coupling between the curvature vector $\boldsymbol{\kappa}$ and the vector part of the interface shape, i.e. the polarization $\mathbf{p}$. Since the toroid is symmetric with respect to a reflection about its plane, spanned by the tangent vector $\hat{\mathbf{t}}$ and normal vector $\hat{\mathbf{n}}$, the coupling between $\mathbf{p}$ and $\boldsymbol{\kappa}$ in the free-energy must maintain this symmetry. Thus, the coupling is proportional to the triple product, $(\mathbf{p} \times \hat{\mathbf{t}}) \cdot \boldsymbol{\kappa} = -\kappa\hat{\mathbf{n}} \cdot \mathbf{p}$. As the curvature-polarization coupling term above is the leading-order coupling of polarization to the ring curvature, the remainder of the free-energy is a function of the magnitude $|\mathbf{p}|$ alone. The equilibrium orientation of the polarization $\mathbf{p}$, as found by minimizing the free-energy, must therefore point toward the axis of revolution, i.e. in the $\hat{\mathbf{n}}$ direction, or away, i.e. in the $-\hat{\mathbf{n}}$ direction; such a configuration is shown in Fig. S.6. This allows us to set $\mathbf{p} = -p\hat{\mathbf{n}}$. Additionally, the same symmetry argument informs coupling of the polarization to the bending strain, proportional to the change in curvature $\Delta\boldsymbol{\kappa}$. Therefore, we conclude that the swelling torque $\mathbf{M}$ that is described in the manuscript is proportional to the polarization: $|\mathbf{M}| \propto p$.

In order to show that the ring curvature of the toroid leads to a solvent distribution where the polymer-dense region is near the axis of revolution of the toroid, i.e. where $p > 0$, we consider the change in the free energy of the cylinder in phase-coexistent equilibrium Eq. 2 due to the addition of a ring curvature $\kappa$ and a polarized solvent distribution with polarization $p$. As the addition of these terms lifts the axial symmetry of the cylinder, the homogeneous deformations described by $\Lambda_t$, $\Lambda_\ell$, and $\Lambda_n$ generally acquire inhomogeneous, anisotropic corrections. These corrections are described by a strain tensor $\epsilon$, the scale of which is set by the small parameters $\kappa$ and $p$. Thus, we are able to consider a separation of scales: the phase-separation, resulting in the solvent-rich core surrounded by the solvent-poor shell, is described by the large deformation matrix elements $\{\Lambda_t, \Lambda_\ell, \Lambda_n\}$ and can be approximated by the values obtained in the cylindrical limit of the gel; the small inhomogeneous strain corrections $\epsilon$ can then be worked out in the linear elastic regime. Following this analysis (see [14]), we find that $\mathbf{p}$ aligns in the direction of $\hat{\mathbf{t}} \times \boldsymbol{\kappa} = -\kappa\hat{\mathbf{n}}$. This confirms the

intuition developed in quasistatic deswelling experiments, where the stress of maintaining coexistent phases is minimized if the deswollen phase is located closer to the axis of revolution and the swollen phase is pushed in the opposite direction.

# 6 Linear stability analysis of the ring model

To determine the stability of the planar ring, we parametrize the centerline as

$$\boldsymbol{\gamma}'(s) = R\left(\cos\frac{s}{R}, \sin\frac{s}{R}, 0\right) + \zeta\left(\frac{s}{R}\right)\hat{\mathbf{b}} = \boldsymbol{\gamma}(s) + \zeta\left(\frac{s}{R}\right)\hat{\mathbf{b}} \tag{7}$$

where $\zeta$ is a small out-of-plane deflection and $\hat{\mathbf{b}} = (0,0,1)$. The resulting Frenet-Serret frame is given by

$$\begin{aligned}
\hat{\mathbf{t}}' &= \frac{\partial_s \boldsymbol{\gamma}'}{|\partial_s \boldsymbol{\gamma}'|} \approx \left(1 - \frac{1}{2}(\partial_s\zeta)^2\right)\hat{\mathbf{t}} + \partial_s\zeta\,\hat{\mathbf{b}} \\
\hat{\mathbf{n}}' &= \frac{\partial_s \hat{\mathbf{t}}'}{|\partial_s \hat{\mathbf{t}}'|} \approx -(\partial_s\zeta)(\partial_{ss}\zeta)\,\hat{\mathbf{t}} + \left(1 - \frac{1}{2}(\partial_{ss}\zeta)^2\right)\hat{\mathbf{n}} + \partial_{ss}\zeta\,\hat{\mathbf{b}} \\
\hat{\mathbf{b}}' &= \hat{\mathbf{t}}' \times \hat{\mathbf{n}}' \approx -\partial_s\zeta\,\hat{\mathbf{t}} - \partial_{ss}\zeta\,\hat{\mathbf{n}} + \left(1 - \frac{1}{2}((\partial_s\zeta)^2 + (\partial_{ss}\zeta)^2)\right)\hat{\mathbf{b}}.
\end{aligned} \tag{8}$$

However, in general, the cross-section orientation can rotate independently of the transverse frame $\{\hat{\mathbf{n}}', \hat{\mathbf{b}}'\}$ [15]; we may express the rotated transverse frame as

$$\begin{pmatrix} \hat{\mathbf{d}}_1 \\ \hat{\mathbf{d}}_2 \end{pmatrix} = \begin{pmatrix} \cos\chi & \sin\chi \\ -\sin\chi & \cos\chi \end{pmatrix} \begin{pmatrix} \hat{\mathbf{n}} \\ \hat{\mathbf{b}} \end{pmatrix}. \tag{9}$$

The curvature is given by $\boldsymbol{\kappa} = \hat{\mathbf{t}} \times \partial_s\hat{\mathbf{t}}$ and the torsion by $\tau = \hat{\mathbf{d}}_2 \cdot \partial_s\hat{\mathbf{d}}_1$; to find the new curvature $\boldsymbol{\kappa}'$ and torsion $\tau'$, derivatives are taken with respect to the new arclength parameter $s'$, where $|\mathrm{d}\boldsymbol{\gamma}'/\mathrm{d}s'| = 1$. The rod free-energy $H$ is given, to second order in $\zeta$ and $\chi$, by

$$H \approx \frac{B}{2R^2}\int_0^{2\pi R} \mathrm{d}s\left[\chi^2 + \frac{C}{B}\left(\partial_{sss}\zeta + \partial_s\zeta + \partial_s\chi\right)^2 - \frac{M}{B\kappa}\left((\partial_{ss}\zeta)^2 - 2(\partial_s\zeta)^2 - \chi^2\right)\right]. \tag{10}$$

Note that choice of angle $\chi$ represents a gauge degree of freedom; it is convenient to choose $\chi = -\partial_{ss}\zeta - \partial_s\zeta + \tilde{\chi}$ so that

$$H \approx \frac{B}{2R^2}\int_0^{2\pi R} \mathrm{d}s\left[\left(1 + \frac{M}{B\kappa}\right)(\partial_{ss}\zeta + \partial_s\zeta - \tilde{\chi})^2 + \frac{C}{B}\left(\partial_s\tilde{\chi}\right)^2 - \frac{M}{B\kappa}\left((\partial_{ss}\zeta)^2 - 2(\partial_s\zeta)^2\right)\right]. \tag{11}$$

Taking advantage of periodic boundary conditions, we expand $\zeta$ and $\tilde{\chi}$ in Fourier modes as

$$\begin{aligned}
\zeta &= \sum_{n=-\infty}^{\infty} \hat{\zeta}_n e^{ins/R}, \quad \hat{\zeta}_{-n} = \hat{\zeta}_n^* \\
\tilde{\chi} &= \sum_{n=-\infty}^{\infty} \hat{\tilde{\chi}}_n e^{ins/R}, \quad \hat{\tilde{\chi}}_{-n} = \hat{\tilde{\chi}}_n^*
\end{aligned} \tag{12}$$

which allows us to write the energy as a quadratic form:

$$H = \sum_{n=-\infty}^{\infty} (\hat{\zeta}_n\ \hat{\tilde{\chi}}_n)^\dagger \mathcal{H}_n (\hat{\zeta}_n\ \hat{\tilde{\chi}}_n) \tag{13}$$

where

$$\mathcal{H}_n = \begin{pmatrix} (n^2-1)^2 + \frac{M}{B\kappa} & \left(1 + \frac{M}{B\kappa}\right)(n^2-1) \\ \left(1 + \frac{M}{B\kappa}\right)(n^2-1) & 1 + \frac{M}{B\kappa} + \frac{C}{B}n^2 \end{pmatrix}. \tag{14}$$

Stability of the planar ring only holds when $\mathcal{H}_n$ is a positive-definite matrix. Thus, the stability threshold is given by

$$\det \mathcal{H}_n = n^2 \left[ \frac{C}{B} \left( \frac{M}{B\kappa} + (n^2-1)^2 \right) - \frac{M}{B\kappa} \left( \frac{M}{B\kappa} + 1 \right) (n^2-2) \right] = 0 \; , \tag{15}$$

which results in the curves shown Fig.4(b) in the manuscript.

We now comment on the validity of the rod model in comparison to the experiments, which show a buckling instability at an aspect ratio of $\xi \approx 3$. While this aspect ratio is rather small for the slender rod approximation used in this model, we expect that the model is qualitatively correct. An indicator of the breakdown of the slender rod approximation comes from a comparison of the extensional energy $E_{\text{ext}} \sim VE(\Delta L/L)^2$, where $\Delta L/L$ is the strain due to changing the length $L$ of the ring by $\Delta L$, with the bending energy $E_{\text{bend}} \sim LB(\Delta\kappa)^2$ [16]. For small strains $\epsilon$, $\Delta L \sim \epsilon L$ and $\Delta\kappa \sim \epsilon/R$. Since length $L \sim R$ and the volume $V \sim Ra^2$, the ratio of the two energies is given by

$$\frac{E_{\text{bend}}}{E_{\text{ext}}} \sim \frac{B}{ER^2a^2} \; . \tag{16}$$

In terms of the Young's modulus $E$, the bending modulus $B$ scales with the second moment of area, $B \sim Ea^4$, so

$$\frac{E_{\text{bend}}}{E_{\text{ext}}} \sim \frac{a^2}{R^2} = \xi^{-2} \; . \tag{17}$$

Therefore, at $\xi = 3$, the bending energy is expected to be almost an order of magnitude smaller than the extensional energy.

# References


[1] Ya-Wen Chang, Alexandros A Fragkopoulos, Samantha M Marquez, Harold D Kim, Thomas E Angelini, and Alberto Fernández-Nieves. Biofilm formation in geometries with different surface curvature and oxygen availability. *New J. Phys.*, 17(3):033017, 2015.

[2] E Pairam, H Le, and A Fernández-Nieves. Stability of toroidal droplets inside yield stress materials. *Phys. Rev. E.*, 90(2):021002, 2014.

[3] R. D. Groot and P. B. Warren. Dissipative particle dynamics: Bridging the gap between atomistic and mesoscopic simulation. *Journal of Chemical Physics*, 107(11):4423–4435, 1997.

[4] P. J. Hoogerbrugge and J. M. V. A. Koelman. Simulating microscopic hydrodynamic phenomena with dissipative particle dynamics. *Europhysics Letters*, 19(3):155–160, 1992.

[5] P. Español and P. Warren. Statistical-mechanics of dissipative particle dynamics. *Europhysics Letters*, 30(4):191–196, 1995.

[6] S. Nikolov, A. Fernández-Nieves, and A. Alexeev. Mesoscale modeling of microgel mechanics and kinetics through the swelling transition. *Applied Mathematics and Mechanics*, 39(1):47–62, 2018.

[7] Toyoichi Tanaka and David J. Fillmore. Kinetics of swelling of gels. *J. Chem. Phys.*, 70(3):1214–1218, 1979.

[8] Paul J. Flory and John Rehner Jr. Statistical mechanics of cross-linked polymer networks i. rubberlike elasticity. *J. Chem. Phys.*, 11(11):512–520, 1943.

[9] Paul J. Flory and John Rehner Jr. Statistical mechanics of cross-linked polymer networks ii. swelling. *J. Chem. Phys.*, 11(11):521–526, 1943.

[10] Masao Doi. Gel dynamics. *Journal of the Physical Society of Japan*, 78(5):052001, 2009.

[11] B. Erman and P. J. Flory. Critical phenomena and transitions in swollen polymer networks and in linear macromolecules. *Macromolecules*, 19(9):2342–2353, 1986.

[12] S. Hirotsu. *Coexistence of phases and the nature of first-order phase transition in poly-N-isopropylacrylamide gels*, pages 1–26. Springer, Berlin, Heidelberg, 1993.

[13] H. B. Callen. *Thermodynamics and an Introduction to Thermostatistics*. Wiley, 1985.

[14] M. S. Dimitriyev. *Function through form in soft matter: the influence of bounded geometries in heated gels and fluctuating proteins*. PhD thesis, Georgia Institute of Technology, School of Physics, 2017.

[15] B. Audoly and Y. Pomeau. *Elasticity and Geometry: From hair curls to the non-linear response of shells*. OUP Oxford, 2010.

[16] L.D. Landau, E.M. Lifshitz, A.M. Kosevich, and L.P. Pitaevskiĭ. *Theory of Elasticity*. Butterworth-Heinemann, New York, 1986.
